# Supplementary material for: Holistic Adversarially Robust Pruning
Source: arXiv:2412.14714 source file (2024-12-19)
Supplement: Supplementary file 1 [file supplementary.tex]

\section{Supplementary}

\subsection{Extended Comparative Evaluation}
\label{app:compare}

We begin by complementing the comparative analysis to \radmm for
both \tradesat and \martat, before we provide a systematic overview of
\ourmethod's result on the small-scale dataset \svhn and the large-scale
dataset \imagenet in comparison to \radmm, and \hydra.

\paragraph{Comparison to \radmm using \tradesat and \martat}
% .
In our experiments summarized in \cref{tab:compare-radmm}, we have
confirmed \radmm's effectivity in coarse-grained and fine-grained robust
pruning based on \pgd adversarial training~\citep{Ye2019Adversarial},
but have shown that our method, \ourmethod, can further improve
performance.
% .
We complement the comparative evaluation by additionally inspecting
\tradesat and \martat to replace the default \pgd loss.
\cref{tab:compare-radmm-rest} shows that in both situations, \radmm
yields similar performance in channel pruning and moderate weight
pruning for \pgdat as reported in \cref{tab:compare-radmm}. However, we
observe a dramatic degradation when pruning weights aggressively.
% .
% Recall \cref{tab:compare-hydra}, \radmm presents a promising
% performance in channel pruning.
Moreover, \radmm preserves natural performance better than robustness.
This can most evidently be seen when pruning channels of \vgg with
\martat, where it achieves exceptionally high natural accuracy but
sacrifices adversary robustness significantly.
% .
In contrast, \ourmethod matches the overwhelming performance of \radmm.
For a weight sparsity of \perc{99.9} in \vgg, our method even yields a
similar model performance as \radmm in \perc{99} sparsity, that is, the
model is an order of magnitude smaller at the same adversarial
robustness.

\begin{table}[tbh]
	\centering
	%\captionsetup{width=0.8\linewidth}
	\caption{Comparing \ourmethod with \radmm on \cifar[10]
		using \tradesat and \martat.}
	
\newcommand{\mycsvreader}[5]{%
	\csvreader[
	head to column names,
	head to column names prefix = COL,
	filter = \equal{\COLarch}{#2} \and \equal{\COLat}{#3} \and 
	\equal{\COLrate}{#4} \and \equal{\COLacc}{#5}
	]%
	{#1}%
	{}
	{
		& \COLradmmbf
		& \COLharpbfradmm
	}
}

\begin{radmmresulttable}{\linewidth}
\midrule
  \multirow{8}{*}{\rotatebox{90}{\resnet[18]}}
& \multirow{4}{*}{\makecell{\trades\\\num{81.30}\,/\,\num{53.21}}}
& --
  \mycsvreader{results/cifar10_weight.csv}{resnet}{trades}{0.99}{nat}
  \mycsvreader{results/cifar10_weight.csv}{resnet}{trades}{0.999}{nat}
  \mycsvreader{results/cifar10_channel.csv}{resnet}{trades}{0.25}{nat}
  \mycsvreader{results/cifar10_channel.csv}{resnet}{trades}{0.1}{nat} 
\\
&
& \fgsm
  \mycsvreader{results/cifar10_weight.csv}{resnet}{trades}{0.99}{fgsm}
  \mycsvreader{results/cifar10_weight.csv}{resnet}{trades}{0.999}{fgsm}
  \mycsvreader{results/cifar10_channel.csv}{resnet}{trades}{0.25}{fgsm}
  \mycsvreader{results/cifar10_channel.csv}{resnet}{trades}{0.1}{fgsm}
\\
&
& \pgd-10
  \mycsvreader{results/cifar10_weight.csv}{resnet}{trades}{0.99}{pgd}
  \mycsvreader{results/cifar10_weight.csv}{resnet}{trades}{0.999}{pgd}
  \mycsvreader{results/cifar10_channel.csv}{resnet}{trades}{0.25}{pgd}
  \mycsvreader{results/cifar10_channel.csv}{resnet}{trades}{0.1}{pgd}
\\
&
& \cwinf
  \mycsvreader{results/cifar10_weight.csv}{resnet}{trades}{0.99}{cw}
  \mycsvreader{results/cifar10_weight.csv}{resnet}{trades}{0.999}{cw}
  \mycsvreader{results/cifar10_channel.csv}{resnet}{trades}{0.25}{cw}
  \mycsvreader{results/cifar10_channel.csv}{resnet}{trades}{0.1}{cw}
\\ \cmidrule{2-11}
& \multirow{4}{*}{\makecell{\mart\\\num{80.16}\,/\,\num{53.72}}}
& --
\mycsvreader{results/cifar10_weight.csv}{resnet}{mart}{0.99}{nat}
\mycsvreader{results/cifar10_weight.csv}{resnet}{mart}{0.999}{nat}
\mycsvreader{results/cifar10_channel.csv}{resnet}{mart}{0.25}{nat}
\mycsvreader{results/cifar10_channel.csv}{resnet}{mart}{0.1}{nat} 
\\
&
& \fgsm
\mycsvreader{results/cifar10_weight.csv}{resnet}{mart}{0.99}{fgsm}
\mycsvreader{results/cifar10_weight.csv}{resnet}{mart}{0.999}{fgsm}
\mycsvreader{results/cifar10_channel.csv}{resnet}{mart}{0.25}{fgsm}
\mycsvreader{results/cifar10_channel.csv}{resnet}{mart}{0.1}{fgsm}
\\
&
& \pgd-10
\mycsvreader{results/cifar10_weight.csv}{resnet}{mart}{0.99}{pgd}
\mycsvreader{results/cifar10_weight.csv}{resnet}{mart}{0.999}{pgd}
\mycsvreader{results/cifar10_channel.csv}{resnet}{mart}{0.25}{pgd}
\mycsvreader{results/cifar10_channel.csv}{resnet}{mart}{0.1}{pgd}
\\
&
& \cwinf
\mycsvreader{results/cifar10_weight.csv}{resnet}{mart}{0.99}{cw}
\mycsvreader{results/cifar10_weight.csv}{resnet}{mart}{0.999}{cw}
\mycsvreader{results/cifar10_channel.csv}{resnet}{mart}{0.25}{cw}
\mycsvreader{results/cifar10_channel.csv}{resnet}{mart}{0.1}{cw}
\\ \midrule
% %%%%%%%%%%%%%%%%%%%%%%%%%
% %%%%%%%%%%%%%%%%%%%%%%%%%
  \multirow{8}{*}{\rotatebox{90}{\vgg}}
& \multirow{4}{*}{\makecell{\trades\\\num{80.18}\,/\,\num{49.72}}}
& --
  \mycsvreader{results/cifar10_weight.csv}{vgg}{trades}{0.99}{nat}
  \mycsvreader{results/cifar10_weight.csv}{vgg}{trades}{0.999}{nat}
  \mycsvreader{results/cifar10_channel.csv}{vgg}{trades}{0.25}{nat}
  \mycsvreader{results/cifar10_channel.csv}{vgg}{trades}{0.1}{nat}
\\
&
& \fgsm
  \mycsvreader{results/cifar10_weight.csv}{vgg}{trades}{0.99}{fgsm}
  \mycsvreader{results/cifar10_weight.csv}{vgg}{trades}{0.999}{fgsm}
  \mycsvreader{results/cifar10_channel.csv}{vgg}{trades}{0.25}{fgsm}
  \mycsvreader{results/cifar10_channel.csv}{vgg}{trades}{0.1}{fgsm}
\\
&
& \pgd-10
  \mycsvreader{results/cifar10_weight.csv}{vgg}{trades}{0.99}{pgd}
  \mycsvreader{results/cifar10_weight.csv}{vgg}{trades}{0.999}{pgd}
  \mycsvreader{results/cifar10_channel.csv}{vgg}{trades}{0.25}{pgd}
  \mycsvreader{results/cifar10_channel.csv}{vgg}{trades}{0.1}{pgd}
\\
&
& \cwinf
  \mycsvreader{results/cifar10_weight.csv}{vgg}{trades}{0.99}{cw}
  \mycsvreader{results/cifar10_weight.csv}{vgg}{trades}{0.999}{cw}
  \mycsvreader{results/cifar10_channel.csv}{vgg}{trades}{0.25}{cw}
  \mycsvreader{results/cifar10_channel.csv}{vgg}{trades}{0.1}{cw}
\\ \cmidrule{2-11}
& \multirow{4}{*}{\makecell{\mart\\\num{73.44}\,/\,\num{51.51}}}
& --
\mycsvreader{results/cifar10_weight.csv}{vgg}{mart}{0.99}{nat}
\mycsvreader{results/cifar10_weight.csv}{vgg}{mart}{0.999}{nat}
\mycsvreader{results/cifar10_channel.csv}{vgg}{mart}{0.25}{nat}
\mycsvreader{results/cifar10_channel.csv}{vgg}{mart}{0.1}{nat}
\\
&
& \fgsm
\mycsvreader{results/cifar10_weight.csv}{vgg}{mart}{0.99}{fgsm}
\mycsvreader{results/cifar10_weight.csv}{vgg}{mart}{0.999}{fgsm}
\mycsvreader{results/cifar10_channel.csv}{vgg}{mart}{0.25}{fgsm}
\mycsvreader{results/cifar10_channel.csv}{vgg}{mart}{0.1}{fgsm}
\\
&
& \pgd-10
\mycsvreader{results/cifar10_weight.csv}{vgg}{mart}{0.99}{pgd}
\mycsvreader{results/cifar10_weight.csv}{vgg}{mart}{0.999}{pgd}
\mycsvreader{results/cifar10_channel.csv}{vgg}{mart}{0.25}{pgd}
\mycsvreader{results/cifar10_channel.csv}{vgg}{mart}{0.1}{pgd}
\\
&
& \cwinf
\mycsvreader{results/cifar10_weight.csv}{vgg}{mart}{0.99}{cw}
\mycsvreader{results/cifar10_weight.csv}{vgg}{mart}{0.999}{cw}
\mycsvreader{results/cifar10_channel.csv}{vgg}{mart}{0.25}{cw}
\mycsvreader{results/cifar10_channel.csv}{vgg}{mart}{0.1}{cw}
\\
\bottomrule
\end{radmmresulttable}
	\label{tab:compare-radmm-rest}
\end{table}

% \begin{wraptable}{r}{0.38\textwidth}
% 	\vspace*{-4mm}
% 	\begin{svhnpretraintable}{\linewidth}
% 		\midrule
% 		\pgd	& 92.40 & 55.09 & 92.70 & 59.33 \\
% 		\trades	& 90.27 & 56.96 & 92.48 & 65.70 \\
% 		\mart	& 89.25 & 56.50 & 92.01 & 62.46 \\
% 		\bottomrule
% 	\end{svhnpretraintable}
% \end{wraptable}

\paragraph{Comparison to \radmm and \hydra on \svhn}

% .
Next, we systematically evaluate \ourmethod on the small-scale \svhn
dataset and present results in \cref{tab:compare-svhn}. The different
rows mention the used adversarial training losses in model's 
pre-train, with the natural accuracy and the \pgd-10
adversarial robustness left and right of the \texttt{/} character,
respectively. %, underneath it.
% .
\hydra again has the upper hand for weight pruning, while \radmm is
better suitable for pruning channels. \ourmethod, in turn, surpasses
both in robustly pruning models learned on \svhn. Both \hydra and \radmm
cause a dramatic drop in the model's performance for aggressive pruning,
while \ourmethod steadily achieves much less robustness degradation even
in this exceptionally challenging setting.

\clearpage

\begin{table}[!h]
	\centering
	%\caption{Comparing \ourmethod's robust pruning with \radmm and 
	%\hydra at \svhn}
	\vspace*{-2mm}
	\caption{Comparing \ourmethod with \radmm and \hydra learned on
		\svhn in pruning weights with \perc{99} and \perc{99.9}
		sparsity~(top), and channels with \perc{75} and \perc{90}
		sparsity~(bottom).}
	
	%\vspace{-0.4cm}
	\begin{subtable}{\linewidth}
		\centering
		%\caption{Weight pruning}
		\newcommand{\mycsvreader}[4]{%
	\csvreader[
	head to column names,
	head to column names prefix = COL,
	filter = \equal{\COLarch}{#1} \and \equal{\COLat}{#2} \and 
	\equal{\COLrate}{#3} \and \equal{\COLacc}{#4}
	]%
	{results/svhn_weight.csv}%
	{}
	{
		& \COLradmmbf
		& \COLhydrabf
		& \COLharpbf
	}
}

\newcommand{\mymidrule}{\cmidrule{2-10}}

\begin{svhnweighttable}{0.96\linewidth}
	\midrule
	\multirow{12}{*}{\rotatebox{90}{\resnet[18]}}
	& \multirow{4}{*}{\makecell{\pgd\\\num{92.70}\,/\,\num{59.33}}}
	%& \multirow{4}{*}{\pgd}
	& --
	\mycsvreader{resnet}{pgd}{0.99}{nat} &
	\mycsvreader{resnet}{pgd}{0.999}{nat} \\
	& & \fgsm
	\mycsvreader{resnet}{pgd}{0.99}{fgsm} &
	\mycsvreader{resnet}{pgd}{0.999}{fgsm} \\
	& & \pgd
	\mycsvreader{resnet}{pgd}{0.99}{pgd} &
	\mycsvreader{resnet}{pgd}{0.999}{pgd} \\
	& & \cwinf
	\mycsvreader{resnet}{pgd}{0.99}{cw} &
	\mycsvreader{resnet}{pgd}{0.999}{cw} \\
	\mymidrule
	%%%%%%%%%%%%%%%%%%%%%%%
	%%%%%%%%%%%%%%%%%%%%%%%
	& \multirow{4}{*}{\makecell{\trades\\\num{92.48}\,/\,\num{65.70}}}
	%& \multirow{4}{*}{\trades}
	& --
	\mycsvreader{resnet}{trades}{0.99}{nat} & 
	\mycsvreader{resnet}{trades}{0.999}{nat} \\
	& & \fgsm
	\mycsvreader{resnet}{trades}{0.99}{fgsm} &
	\mycsvreader{resnet}{trades}{0.999}{fgsm} \\
	& & \pgd
	\mycsvreader{resnet}{trades}{0.99}{pgd} &
	\mycsvreader{resnet}{trades}{0.999}{pgd} \\
	& & \cwinf
	\mycsvreader{resnet}{trades}{0.99}{cw} &
	\mycsvreader{resnet}{trades}{0.999}{cw} \\
	\mymidrule
	%%%%%%%%%%%%%%%%%%%%%%%
	%%%%%%%%%%%%%%%%%%%%%%%
	& \multirow{4}{*}{\makecell{\mart\\\num{92.01}\,/\,\num{62.46}}}
	%& \multirow{4}{*}{\mart}
	& --
	\mycsvreader{resnet}{mart}{0.99}{nat} & 
	\mycsvreader{resnet}{mart}{0.999}{nat} \\
	& & \fgsm
	\mycsvreader{resnet}{mart}{0.99}{fgsm} &
	\mycsvreader{resnet}{mart}{0.999}{fgsm} \\
	& & \pgd
	\mycsvreader{resnet}{mart}{0.99}{pgd} &
	\mycsvreader{resnet}{mart}{0.999}{pgd} \\
	& & \cwinf
	\mycsvreader{resnet}{mart}{0.99}{cw} &
	\mycsvreader{resnet}{mart}{0.999}{cw} \\
	%%%%%%%%%%%%%%%%%%%%%%%%%%%%%%%%%%%%%%%%%%%%%%%%%%%%%%%%%%%%
	%%%%%%%%%%%%%%%%%%%%%%%%%%%%%%%%%%%%%%%%%%%%%%%%%%%%%%%%%%%%
	%%%%%%%%%%%%%%%%%%%%%%%%%%%%%%%%%%%%%%%%%%%%%%%%%%%%%%%%%%%%
	\midrule
	\multirow{12}{*}{\rotatebox{90}{\vgg}}
	& \multirow{4}{*}{\makecell{\pgd\\\num{92.40}\,/\,\num{55.09}}}
	%& \multirow{4}{*}{\pgd}
	& --
	\mycsvreader{vgg}{pgd}{0.99}{nat} &
	\mycsvreader{vgg}{pgd}{0.999}{nat} \\
	& & \fgsm
	\mycsvreader{vgg}{pgd}{0.99}{fgsm} &
	\mycsvreader{vgg}{pgd}{0.999}{fgsm} \\
	& & \pgd
	\mycsvreader{vgg}{pgd}{0.99}{pgd} &
	\mycsvreader{vgg}{pgd}{0.999}{pgd} \\
	& & \cwinf
	\mycsvreader{vgg}{pgd}{0.99}{cw} &
	\mycsvreader{vgg}{pgd}{0.999}{cw} \\
	\mymidrule
	%%%%%%%%%%%%%%%%%%%%%%%
	%%%%%%%%%%%%%%%%%%%%%%%
	& \multirow{4}{*}{\makecell{\trades\\\num{90.27}\,/\,\num{56.96}}}
	%& \multirow{4}{*}{\trades}
	& --
	\mycsvreader{vgg}{trades}{0.99}{nat} &
	\mycsvreader{vgg}{trades}{0.999}{nat} \\
	& & \fgsm
	\mycsvreader{vgg}{trades}{0.99}{fgsm} &
	\mycsvreader{vgg}{trades}{0.999}{fgsm} \\
	& & \pgd
	\mycsvreader{vgg}{trades}{0.99}{pgd} &
	\mycsvreader{vgg}{trades}{0.999}{pgd} \\
	& & \cwinf
	\mycsvreader{vgg}{trades}{0.99}{cw} &
	\mycsvreader{vgg}{trades}{0.999}{cw} \\
	\mymidrule
	%%%%%%%%%%%%%%%%%%%%%%%
	%%%%%%%%%%%%%%%%%%%%%%%
	& \multirow{4}{*}{\makecell{\mart\\\num{89.25}\,/\,\num{56.50}}}
	%& \multirow{4}{*}{\mart}
	& --
	\mycsvreader{vgg}{mart}{0.99}{nat} &
	\mycsvreader{vgg}{mart}{0.999}{nat} \\
	& & \fgsm
	\mycsvreader{vgg}{mart}{0.99}{fgsm} &
	\mycsvreader{vgg}{mart}{0.999}{fgsm} \\
	& & \pgd
	\mycsvreader{vgg}{mart}{0.99}{pgd} &
	\mycsvreader{vgg}{mart}{0.999}{pgd} \\
	& & \cwinf
	\mycsvreader{vgg}{mart}{0.99}{cw} &
	\mycsvreader{vgg}{mart}{0.999}{cw} \\
	%\bottomrule
\end{svhnweighttable}
		\label{tab:compare-svhn}
		%\vspace*{-2pt}
		\vspace*{10pt}
	\end{subtable}
	\begin{subtable}{\linewidth}
		\centering
		%\caption{Channel pruning}
		\newcommand{\mycsvreader}[4]{%
	\csvreader[
	head to column names,
	head to column names prefix = COL,
	filter = \equal{\COLarch}{#1} \and \equal{\COLat}{#2} \and 
	\equal{\COLrate}{#3} \and \equal{\COLacc}{#4}
	]%
	{results/svhn_channel.csv}%
	{}
	{
		& \COLradmmbf
		& \COLhydrabf
		& \COLharpbf
	}
}

\newcommand{\mymidrule}{\cmidrule{2-10}}

\begin{svhnchanneltable}{.96\linewidth}
	\midrule
	\multirow{12}{*}{\rotatebox{90}{\resnet[18]}}
	& \multirow{4}{*}{\makecell{\pgd\\\num{92.70}\,/\,\num{59.33}}}
	%& \multirow{4}{*}{\pgd}
	& --
	\mycsvreader{resnet}{pgd}{0.25}{nat} &
	\mycsvreader{resnet}{pgd}{0.1}{nat} \\
	& & \fgsm
	\mycsvreader{resnet}{pgd}{0.25}{fgsm} &
	\mycsvreader{resnet}{pgd}{0.1}{fgsm} \\
	& & \pgd
	\mycsvreader{resnet}{pgd}{0.25}{pgd} &
	\mycsvreader{resnet}{pgd}{0.1}{pgd} \\
	& & \cwinf
	\mycsvreader{resnet}{pgd}{0.25}{cw} &
	\mycsvreader{resnet}{pgd}{0.1}{cw} \\
	\mymidrule
	%%%%%%%%%%%%%%%%%%%%%%%
	%%%%%%%%%%%%%%%%%%%%%%%
	& \multirow{4}{*}{\makecell{\trades\\\num{92.48}\,/\,\num{65.70}}}
	%& \multirow{4}{*}{\trades}
	& --
	\mycsvreader{resnet}{trades}{0.25}{nat} &
	\mycsvreader{resnet}{trades}{0.1}{nat} \\
	& & \fgsm
	\mycsvreader{resnet}{trades}{0.25}{fgsm} &
	\mycsvreader{resnet}{trades}{0.1}{fgsm} \\
	& & \pgd
	\mycsvreader{resnet}{trades}{0.25}{pgd} &
	\mycsvreader{resnet}{trades}{0.1}{pgd} \\
	& & \cwinf
	\mycsvreader{resnet}{trades}{0.25}{cw} &
	\mycsvreader{resnet}{trades}{0.1}{cw} \\
	\mymidrule
	%%%%%%%%%%%%%%%%%%%%%%%
	%%%%%%%%%%%%%%%%%%%%%%%
	& \multirow{4}{*}{\makecell{\mart\\\num{92.01}\,/\,\num{62.46}}}
	%& \multirow{4}{*}{\mart}
	& --
	\mycsvreader{resnet}{mart}{0.25}{nat} &
	\mycsvreader{resnet}{mart}{0.1}{nat} \\
	& & \fgsm
	\mycsvreader{resnet}{mart}{0.25}{fgsm} &
	\mycsvreader{resnet}{mart}{0.1}{fgsm} \\
	& & \pgd
	\mycsvreader{resnet}{mart}{0.25}{pgd} &
	\mycsvreader{resnet}{mart}{0.1}{pgd} \\
	& & \cwinf
	\mycsvreader{resnet}{mart}{0.25}{cw} &
	\mycsvreader{resnet}{mart}{0.1}{cw} \\
	%%%%%%%%%%%%%%%%%%%%%%%%%%%%%%%%%%%%%%%%%%%%%%%%%%%%%%%%%%%%
	%%%%%%%%%%%%%%%%%%%%%%%%%%%%%%%%%%%%%%%%%%%%%%%%%%%%%%%%%%%%
	%%%%%%%%%%%%%%%%%%%%%%%%%%%%%%%%%%%%%%%%%%%%%%%%%%%%%%%%%%%%
		\midrule
	\multirow{12}{*}{\rotatebox{90}{\vgg}}
	& \multirow{4}{*}{\makecell{\pgd\\\num{92.40}\,/\,\num{55.09}}}
	%& \multirow{4}{*}{\pgd}
	& --
	\mycsvreader{vgg}{pgd}{0.25}{nat} &
	\mycsvreader{vgg}{pgd}{0.1}{nat} \\
	& & \fgsm
	\mycsvreader{vgg}{pgd}{0.25}{fgsm} &
	\mycsvreader{vgg}{pgd}{0.1}{fgsm} \\
	& & \pgd
	\mycsvreader{vgg}{pgd}{0.25}{pgd} &
	\mycsvreader{vgg}{pgd}{0.1}{pgd} \\
	& & \cwinf
	\mycsvreader{vgg}{pgd}{0.25}{cw} &
	\mycsvreader{vgg}{pgd}{0.1}{cw} \\
	\mymidrule
	%%%%%%%%%%%%%%%%%%%%%%%
	%%%%%%%%%%%%%%%%%%%%%%%
	& \multirow{4}{*}{\makecell{\trades\\\num{90.27}\,/\,\num{56.96}}}
	%& \multirow{4}{*}{\trades}
	& --
	\mycsvreader{vgg}{trades}{0.25}{nat} &
	\mycsvreader{vgg}{trades}{0.1}{nat} \\
	& & \fgsm
	\mycsvreader{vgg}{trades}{0.25}{fgsm} &
	\mycsvreader{vgg}{trades}{0.1}{fgsm} \\
	& & \pgd
	\mycsvreader{vgg}{trades}{0.25}{pgd} &
	\mycsvreader{vgg}{trades}{0.1}{pgd} \\
	& & \cwinf
	\mycsvreader{vgg}{trades}{0.25}{cw} &
	\mycsvreader{vgg}{trades}{0.1}{cw} \\
	\mymidrule
	%%%%%%%%%%%%%%%%%%%%%%%
	%%%%%%%%%%%%%%%%%%%%%%%
	& \multirow{4}{*}{\makecell{\mart\\\num{89.25}\,/\,\num{56.50}}}
	%& \multirow{4}{*}{\mart}
	& --
	\mycsvreader{vgg}{mart}{0.25}{nat} &
	\mycsvreader{vgg}{mart}{0.1}{nat} \\
	& & \fgsm
	\mycsvreader{vgg}{mart}{0.25}{fgsm} &
	\mycsvreader{vgg}{mart}{0.1}{fgsm} \\
	& & \pgd
	\mycsvreader{vgg}{mart}{0.25}{pgd} &
	\mycsvreader{vgg}{mart}{0.1}{pgd} \\
	& & \cwinf
	\mycsvreader{vgg}{mart}{0.25}{cw} &
	\mycsvreader{vgg}{mart}{0.1}{cw} \\
	\bottomrule
\end{svhnchanneltable}
		\label{tab:compare-svhn-ch}
	\end{subtable}
\end{table}
\clearpage
\clearpage

\subparagraph{Weight pruning} As \hydra uses scores optimization,
\cref{tab:compare-svhn} allows us to judge the impact of using
connection-importance optimization for learning \svhn.
% .
In contrast to channel pruning, \hydra here presents much higher
stability when facing different adversarial training methods. \radmm,
however, is sensitive to weight sparsity, yielding drastic performance
degradation at \perc{99.9} sparsity with \tradesat.
% .
Moreover, \hydra outperforms \radmm in every single weight-pruning
experiment, however, \ourmethod always achieves higher robustness.
Especially, in pruning \perc{99.9} of the network's weights, \ourmethod
manages to maintain \pgd-10 robustness in proximity of \num{10.21}
percentage points, while \hydra's performance degradation is $3\times$
higher.

\subparagraph{Channel pruning} \pgd adversarial training is challenging
for both \hydra and \radmm. For a channel sparsity of \perc{75}, both
show good pruning performance while for a higher sparsity of \perc{90},
\hydra drops in performance and \radmm can only keep up in pruning
\resnet. In contrast, our method can preserve the model's performance in
both moderate and aggressive channel pruning.
% .
However, in comparison with the successful attempts of \radmm,
\ourmethod achieves even higher robustness and natural accuracy.
\hydra's performance loss is particularly striking when using \tradesat
and \martat. Notably, \ourmethod shows better adaptability in both
training methods.
% .
Irrespective of the sparsity, \ourmethod constantly achieves higher
robustness, although sometimes, it trades performance on natural data
for higher robustness.

\iffalse
Overall in \cref{tab:compare-svhn} , \ourmethod realizes the 
combination of advantages in \hydra and \radmm. Meanwhile, it achieves 
the surpass beyond both. Furthermore, \ourmethod presents a significant 
stability and much higher resistance against the harm from pruning, 
which infers a good reliability of our method in the robustness-aware 
model pruning. 

%In contrast to \cifar[10], pruning \svhn faces the challenge of the 
%class-wise imbalance problem~\citep{Zhao2022nonuniform}.
\fi

\paragraph{Strategy analysis on \vgg in \cifar[10]}~

\begin{figure}[!htbp]
	\centering
	\captionsetup{width=0.9\linewidth}
	\caption{Comparing strategies of \ourmethod, \lamp, and 
	\erk in compression rates for pruning weights a \perc{99.9} 
	sparsity on robustly 
	pretrained \vgg by \pgdat in \cifar[10].}% of \pgdat pre-trained 
	%\vgg 
	%model.} 
	\input{figures/compare-lamp-erk-vgg16-stg.tex}
	\label{fig:stg-compare-vgg}\vspace*{-2mm}
\end{figure}

%\paragraph{Strategy analysis on \resnet in \cifar[10]}~
%
%\begin{table}[!htbp]
%	\centering
%	\captionsetup{width=.55\linewidth}
%	\caption{Comparing pruning \resnet weights by 
%	\hydra with \erk and \lamp and by \ourmethod in \cifar[10]}
%	\tablesize
%	\input{tables/stg-compare-resnet.tex}
%\end{table}
%
%\begin{figure}[!htbp]
%	\caption{Compression strategies of \ourmethod, \lamp, and \erk for 
%	pruning 
%		weights a \perc{99.9} sparsity.}% of \pgdat pre-trained \vgg 
%		%model.} 
%	\input{figures/compare-lamp-erk-resnet.tex}
%	\label{fig:stg-overview-resnet}\vspace*{-2mm}
%\end{figure}

\newpage

\begin{figure}[!htbp]
	\centering
	\captionsetup{width=.75\linewidth}
	\caption{Comparing strategies of \ourmethod, \lamp, and \erk in 
	compression rates for pruning \resnet weights a \perc{99.9} 
	sparsity in \cifar[10].}% 
		%of 
		%\pgdat pre-trained \vgg 
	%model.} 
	\input{figures/compare-lamp-erk-resnet-stg.tex}
	\label{fig:stg-compare-resnet}
\end{figure}

\paragraph{Parameter distribution on pruning channels}

\newpage

%\paragraph{Evaluation on \radmm using non-uniform strategies}~
%%
%\begin{table}[!htbp]
%	\vspace*{-4mm}
%	\caption{Comparing weight pruning by using \radmm with \erk and 
%	\lamp and by \ourmethod}
%	\vspace*{-4mm}
%	\tablesize
%	\input{tables/stg-compare-radmm.tex}
%	\vspace*{-2mm}
%\end{table}
%%
%\begin{table}[!htbp]
%	\vspace*{-4mm}
%	\caption{Comparing weight pruning by using \hydra with \erk and 
%		\lamp and by \ourmethod}
%	\vspace*{-4mm}
%	\tablesize
%	\input{tables/stg-compare-hydra.tex}
%	\vspace*{-2mm}
%\end{table}

%\paragraph{Evaluation across end-to-end pruning}~
%%
%\begin{figure}[!tbh]
%	\caption{End-to-end pruning \pgd-10 pre-trained \resnet by 
%	\ourmethod}
%	\captionsetup[subfigure]{oneside, margin={12mm, 0mm}}
%	\begin{subfigure}[h]{.4\linewidth}
%		\caption{Weight Sparsity \perc{99}}
%		\vspace{-2mm}
%		\input{figures/pcurve-resnet-w001.tex}
%		\label{fig:harpprune-resnet-w001}
%	\end{subfigure}
%	\hskip 45pt
%	\begin{subfigure}[h]{.4\linewidth}
%		\caption{Weight Sparsity \perc{99.9}}
%		\vspace{-2mm}
%		\input{figures/pcurve-resnet-w0001.tex}
%		\label{fig:harpprune-resnet-w0001}
%	\end{subfigure}
%	
%%	\begin{subfigure}[h]{.4\linewidth}
%%		\caption{Channel Sparsity \perc{75}}
%%		\vspace{-2mm}
%%		\input{figures/pcurve-resnet-ch025.tex}
%%		\label{fig:harpprune-resnet-ch025}
%%	\end{subfigure}
%%	\hskip 45pt
%%	\begin{subfigure}[h]{.4\linewidth}
%%		\caption{Channel Sparsity \perc{90}}
%%		\vspace{-2mm}
%%		\input{figures/pcurve-resnet-ch01.tex}
%%		\label{fig:harpprune-resnet-ch01}
%%	\end{subfigure}
%\end{figure}

\begin{figure}[!tbh]
	\caption{End-to-end pruning \pgd-10 pre-trained \vgg by \ourmethod}
	\captionsetup[subfigure]{oneside, margin={12mm, 0mm}}
	\begin{subfigure}[h]{.4\linewidth}
		\caption{Weight Sparsity \perc{99}}
		\vspace{-2mm}
		\input{figures/pcurve-vgg-w001.tex}
		\label{fig:harpprune-vgg-w001}
	\end{subfigure}
	\hskip 45pt
	\begin{subfigure}[h]{.4\linewidth}
		\caption{Weight Sparsity \perc{99.9}}
		\vspace{-2mm}
		\input{figures/pcurve-vgg-w0001.tex}
		\label{fig:harpprune-vgg-w0001}
	\end{subfigure}

%	\begin{subfigure}[h]{.4\linewidth}
%		\caption{Channel Sparsity \perc{75}}
%		\vspace{-2mm}
%		\input{figures/pcurve-vgg-ch025.tex}
%		\label{fig:harpprune-vgg-ch025}
%	\end{subfigure}
%	\hskip 45pt
%	\begin{subfigure}[h]{.4\linewidth}
%		\caption{Channel Sparsity \perc{90}}
%		\vspace{-2mm}
%		\input{figures/pcurve-vgg-ch01.tex}
%		\label{fig:harpprune-vgg-ch01}
%	\end{subfigure}
\end{figure}

\begin{table}[!htbp]
	\centering
	\caption{Comparing \ourmethod with \radmm and \hydra learned on
		\imagenet.}
	\newcommand{\mycsvreader}[3]{%
	\csvreader[
	head to column names,
	head to column names prefix = COL,
	filter = \equal{\COLattack}{#1} \and \equal{\COLpreg}{#2} \and 
	\equal{\COLprate}{#3}
	]%
	{results/imagenet_results.csv}%
	{}
	{
		& \COLradmmbf
		& \COLhydrabf
		& \COLharpbf
	}
}

\begin{imagenetablemoderate}{\linewidth}
	\midrule
	% \multirow{7}{*}{\rotatebox{90}{Channel Prune}} & 
	\multirow{4}{*}{\makecell{\bfseries \freeat\\ 
	\num{60.25}\,/\,\num{32.82}}}
	& -- 		
	\mycsvreader{nat}{weight}{0.1} 
	& \mycsvreader{nat}{channel}{0.5}\\
	& \fgsm 	
	\mycsvreader{fgsm}{weight}{0.1} 
	& \mycsvreader{fgsm}{channel}{0.5}\\
	& \pgd-10 	
	\mycsvreader{pgd}{weight}{0.1} 
	& \mycsvreader{pgd}{channel}{0.5}\\
	& \cwinf
	\mycsvreader{cw}{weight}{0.1} 
	& \mycsvreader{cw}{channel}{0.5}\\
	\bottomrule
%	\multirow{7}{*}{\rotatebox{90}{Weight Prune}} 
%	& \multirow{3}{*}{\perc{90}} 
%	\mycsvreader{hydrabf}{weight}{0.1} \\
%	& \mycsvreader{radmmbf}{weight}{0.1} \\ \cmidrule{3-7}
%	& \mycsvreader{harpbf}{weight}{0.1}
%	\\ \cmidrule{2-7}
%	& \multirow{3}{*}{\perc{99}} 
%	\mycsvreader{hydrabf}{weight}{0.01} \\ 
%	& \mycsvreader{radmmbf}{weight}{0.01} \\ \cmidrule{3-7}
%	& \mycsvreader{harpbf}{weight}{0.01}
%	\\ \midrule

\end{imagenetablemoderate}
	\label{tab:compare-imgnet-moderate}
\end{table}
